# Supplementary material for: Closed-book Question Generation via Contrastive Learning
Source: arXiv:2210.06781 source file (2023-02-10)
Supplement: Supplementary file 1 [file appendix.tex]

\section{Question-Type Unigram}
\label{sec:question-type-unigram}
The list of terms used for filtering questions: ``how'', ``what'', ``can'', ``is'', ``do'', ``why'', ``are'', ``does'', ``where'', ``when'', ``should'', ``will'', ``did'', ``which'', ``who'', ``would'', ``if'', ``about'', ``for'', ``as'', ``could'', ``in'', ``after'', ``at'', ``while'', ``to'', ``am'', ``has'', ``any''.

\section{Question Answer Pairs in WikiCQA}

Table~\ref{tab:qa-examples} shows the question-answer pairs in our WikiCQA dataset.

\begin{table*}[htbp!]
\centering
\begin{tabular}{p{0.3\textwidth}p{0.6\textwidth}}
\hline
\textbf{Questions} & \textbf{Answers} \\
\hline
What is the easiest nut to grow? & The American hazelnut is one of the easiest nuts to grow, so you could try that one. \\
Can you lose weight by swimming? & Yes, as long as you maintain a balanced calorie controlled diet, you can lose weight by swimming. \\
How long will red lentils keep for in the pantry? & Properly stored in an airtight container, the red lentils should keep for up to a year. \\
Is euphorbia a perennial? & Yes, euphorbia is considered a perennial, meaning it will grow back year after year. \\
\hline
\end{tabular}
\caption{Question-answer pairs in WikiCQA.}
\label{tab:qa-examples}
\end{table*}

\section{More Examples for Question Generation}

Table~\ref{tab:qg-examples} shows the generated questions from our best model.

\begin{table*}[hb!]
\centering
\begin{tabular}{p{1cm}p{0.85\textwidth}}
\hline
\textbf{A} & Recovery time varies depending on your age and how deeply the teeth were impacted. Some people recover quickly within 48 hours to four days, while some people find it can take up to a week or so... \\
\textbf{B-Q} & \\
\textbf{G-Q} & How long does it take to recover from wisdom teeth removal? \\
\textbf{GT-Q} & How many days does it take to recover from wisdom tooth removal? \\
\hline
\end{tabular}
\caption{Generated questions from our best model.}
\label{tab:qg-examples}
\end{table*}

\section{More Examples for Question Answering}

% To teach your dog to track, start by teaching it to sit and stay so it can develop the patience needed for tracking. While your dog is seated in one place, show it one of its favorite toys, then allow your dog to watch you place it somewhere in plain sight. After that, practice commanding your dog to retrieve the toy, using a common cue like “seek.” When it has the toy in its mouth, run back to the starting position and encourage your dog to follow. Then, tell your dog to drop the toy and reward it immediately after each successful retrieval. 

Figure~\ref{tab:summary-example} shows an example from the WikiHow.
\begin{table*}[htbp!]
\centering
\begin{tabular}{p{0.95\textwidth}}
\hline
\textbf{Title:} How to Prepare a Healthy Meal for Your Pet Dog \\
\textbf{Summary:} To prepare a healthy meal for your dog, choose lean meat with the bones and fat removed, like chicken or beef, since this should make up 50 percent of the meal. The other half of the meal should be made up equally of carbohydrates and vegetables so your dog gets a variety of nutrients. Some good options to consider are rice or pasta for carbohydrates, and broccoli, zucchini, or squash for vegetables. If you want to give your dog some extra protein, try to add one egg for every 20 pounds your dog weighs, or you may overfeed it. \\ \hline
\textbf{Question:} What can I feed my dog if I have run out of dog food? \\
\textbf{Answer:} In the short term, any bland human food such as chicken or white fish with rice or pasta is just fine. This will tide the dog over until you can get to the store, but isn't nutritionally balanced for long term feeding. \\
\textbf{Question:} How much homemade dog food do you feed your dog? \\
\textbf{Answer:} Great question because it highlights one of the problems of feeding home prepared foods. Each food contains a different number of calories, so you need to feed different amounts depending on the individual recipe and there's no one-size-fits-all answer. \\
\textbf{Question:} What should I not feed my dog?  \\
\textbf{Answer:} There are many human foods that are toxic to dogs. Top of the list of foods NOT to give are grapes, raisins, chocolate, onions, and garlic. Also dangerous to dogs is any product containing xylitol. In short, if you aren't sure, always check if a new food is safe before giving it to a dog. \\

\hline
\end{tabular}
\caption{Question-answer pairs from WikiHow.}
\label{tab:summary-example}
\end{table*}

\begin{table*}[htbp!]
\centering
\begin{tabular}{cccccccc}
\hline
\textbf{Models} & \textbf{R-1} & \textbf{R-2} & \textbf{R-L} & \textbf{R-LSum} & \textbf{BLEU} & \textbf{BERTScore} & \textbf{METEOR}\\
\hline
QG & 48.39 & 26.84 & 46.08 & 46.16 & 18.52& 58.63 & 44.79 \\
QG-cl-t & 48.67 & 27.34 & 46.43 & 46.46 & 18.96 & 58.57 & 45.37 \\
QG-cl-s & 48.72 & 27.26 & 46.33 & 46.41 & 19.06 & 58.37 & 45.41 \\
QG-cl-t-qa & \textbf{49.26} & 27.77 & 46.82 & 46.88 & 19.09 & \textbf{58.99} & \textbf{45.58} \\
QG-cl-s-qa & 49.22 & \textbf{27.79} & \textbf{46.98} & \textbf{47.08} & \textbf{19.21} & 58.92 & 45.40 \\
\hline
\end{tabular}
\caption{QG results.}
\label{tab:appendix-qg-results}
\end{table*}

\begin{table*}
\centering\small
\begin{tabular}{ccccccccc}
\hline
\textbf{Dataset} & \textbf{Model} & \textbf{R1} & \textbf{R2} & \textbf{RougeL} & \textbf{RougnLsum} & \textbf{BLEU} & \textbf{BERTScore} & \textbf{METEOR}   \\
\hline
\multirow{3}{*}{WikiCQA} & BART-base & 27.16 & 7.32 & 19.85 & 23.49 & 3.06 & 26.27 & 18.11 \\
                         & QG-no fine-tuning & 24.10 & 7.07 & 18.02 & 20.31 & 1.68 & 25.10 & 15.09 \\
                         & QG-fine-tuned & \textbf{28.44} & \textbf{8.14} & \textbf{20.56} & \textbf{24.77} & \textbf{3.69} & \textbf{26.89} & \textbf{19.62} \\ \hline
\multirow{3}{*}{GooAQ} & BART-base & 27.72 & 7.68 & 20.08 & 23.64 & 3.30 & 20.64 & 17.27 \\
                      & QG-no fine-tuning & 21.93 & 6.12 & 16.62  & 18.35 & 0.76 & 16.62 & 12.12 \\
                      & QG-fine-tuned & \textbf{28.44} & \textbf{7.73} & \textbf{20.17} & \textbf{24.12} & \textbf{3.74} & 19.66 & \textbf{18.35} \\ \hline
\multirow{3}{*}{ELI5} & BART-base & 22.06 & 3.93 & 13.93 & 19.72 & 1.56 & 6.55 & 14.92 \\
                      & QG-no fine-tuning & 13.97 & 2.29 & 10.00 & 11.77 & 0.06 & 6.17 & 7.45 \\
                      & QG-fine-tuned     &         &        &         &           &        &           &         \\
\hline
\end{tabular}
\caption{QA results.}
\label{tab:appendix-qa-results}
\end{table*}
